# Supplementary material for: Erbium-Doped Fibre Quantum Memory for Chip-Integrated Quantum-Dot Single Photons at 980 nm
Source: arXiv:2508.01416 ancillary file (2025-08-02)
Supplement: Supplementary file 1 [file SupplementaryInformation.pdf]

# Supplementary Information for: Erbium-Doped Fibre Quantum Memory for Chip-Integrated Quantum-Dot Single Photons at 980 nm

Nasser Gohari Kamel[1,2,*] Arsalan Mansourzadeh[1,2,*] Ujjwal Gautam[1,2], Vinaya Kumar Kavatamane[1,2], Ashutosh Singh[1,2], Edith Yeung[3,4], David B. Northeast[4], Paul Barclay[1,2], Philip J. Poole[4], Dan Dalacu[3,4], and Daniel Oblak[1,2†]
[1]*Institute for Quantum Science and Technology, University of Calgary, Calgary, AB, Canada T2N 1N4*
[2]*Department of Physics and Astronomy, University of Calgary, Calgary, AB, Canada T2N 1N4*[‡]
[3]*Department of Physics, University of Ottawa, Ottawa, Ontario, Canada K1N 6N5 and*
[4]*National Research Council Canada, Ottawa, ON, Canada K1A 0R6*
(Dated: August 1, 2025)

In this Supplementary Information, we present additional experimental results of atomic frequency comb (AFC) quantum memory (QM) implementation utilizing 980 nm optical transition of erbium-doped glass silica fibers (EDF) under three distinct magnetic field conditions. We demonstrate the QM performance for storage and retrieval of a weak coherent pulse for varying storage durations. The electronic connection diagram is presented, providing more insight into the experimental setup. Lastly, we introduce our methodology for tailoring the inhomogeneous broadening, enabling the preparation of 8 GHz-wide AFCs with tunable predetermined storage times, thus advancing the versatility and applicability of AFC-based QMs.

## A. QM performance vs magnetic field

EDFs exhibit distinctive properties (wide inhomogeneous broadening and long spin lifetimes) that position them as highly promising candidates for the implementation of broadband QM applications. We investigate the AFC QM performance implemented on EDF at 980 nm at three different magnetic fields for different storage times up to 100 ns. All AFCs are prepared with the same 8 GHz bandwidth, while only one weak coherent probe pulse with 320 ps temporal duration is stored and recalled. We repeat the experiment four times and take the average of echo intensities (SNSPD counts) for each storage duration. Our results demonstrate that the efficiency of the recalled echo at each magnetic field depends on the optical coherence time. We observe that the efficiency of the echo is slightly higher at $B = 0.06$ T compared to 0.03 T and 0.09 T.

The experimental results are depicted in FIG. S1, where we observe an oscillatory behavior in the recalled echo intensity vs. storage time. To prepare the AFC combs, based on the desired storage time, we generate a train of optical pulses with a 50% duty cycle, lasting for a duration of $T$. Simultaneously, the frequency of this pulse train is linearly swept across the entire bandwidth of the AFC (see Section C for more details). In this approach, the frequency of each optical pulse varies according to its position within the pulse train. For instance, the first pulse undergoes a frequency shift to -3.8 GHz, while the last pulse shifts to +4.2 GHz. To ensure optimal overlap between the bandwidths of the weak coherent probe pulses and the AFC comb, we apply a linear frequency sweep from $\nu_0 - 3.8$ GHz to $\nu_0 + 4.2$ GHz. However, since the phase modulator (PM) does not operate perfectly with the frequency shift to only one sideband, a slightly unwanted frequency shift from the opposite order will also be present. This unwanted opposite order sometimes results in optical pumping of the absorbing teeth and reduces the effective optical depth (OD) of the AFC. Therefore, the main reason for observing the fluctuation of the recalled echoes vs storage time is the variation of the effective OD. In another experiment, we changed the offset frequency to 100 MHz (3.9 GHz to 4.1 GHz), and the periodicity of echo amplitudes increased to 30 ns (the results are not depicted here). Another reason for this fluctuation could be due to the interference of the echo with any possible leak light from the IM, resulting in constructive and destructive interference.

## B. Electrical connections in experimental setup

The experimental setup in the main text (see [1]) only represents optical components that are utilized in this research. In addition, it is worth describing the electrical connection diagram (see FIG. S2) that drives the different optical components. Here an Arbitrary Waveform Generator (AWG, Tektronix 70002A) with two analog channels (and four marker channels) is utilized to drive the first Acousto Optic Modulator (AOM, RF drive frequency of 200 MHz) and a 980 nm PM in which is derived with serrodyne RF signals to create a single side-band optical frequency shift. The first MEMs switch on the input port is derived with a trigger signal generated from a marker channel of AWG and the first delay generator delay $\text{gen}_1$. The second delay $\text{gen}_2$, upon receiving the trigger signal from another marker channel on AWG, generates a TTL signal for the RF switch and then a trigger signal for the Arbitrary Function Generator (AFG). The input to the RF switch is supplied from an 85 MHz RF source, to drive the second AOM. Upon receiving the trigger from

* These authors contributed equally.
† doblak@ucalgary.ca
‡ https://qcloudlab.com/

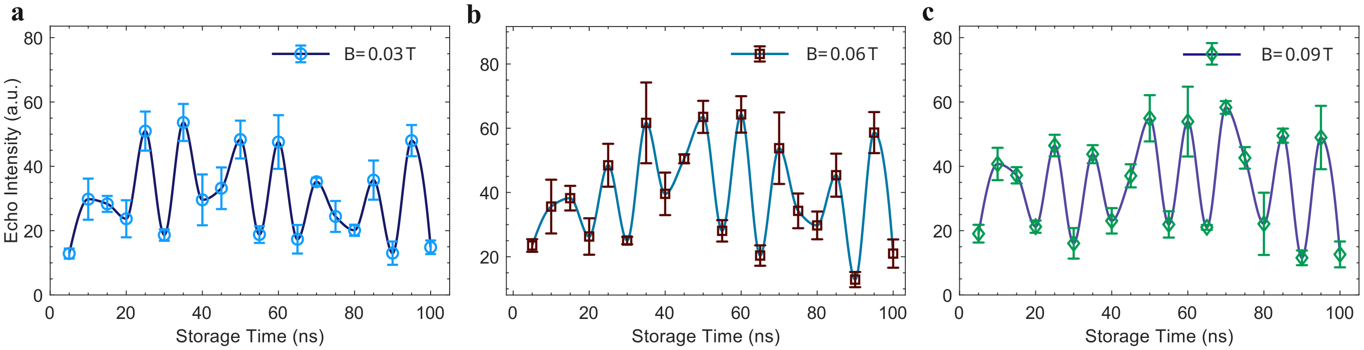


FIG. S1. **AFC QM performance.** Here, a weak probe pulse is stored and recalled at three different magnetic fields of **a,** 0.03 T, **b,** 0.06 T, and **c,** 0.09 T.

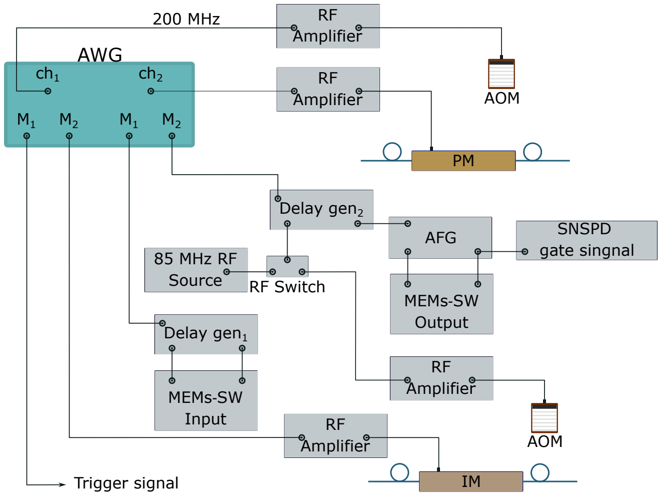


FIG. S2. **Electrical connection diagram.** Here, AWG is the core component from which all the optical components are derived based on the timings set accordingly. We use AFG for 85 MHz RF source, RF amplifiers for IM and PM (iXble, DR-VE-10-MO), RF amplifiers for AOMs (mini circuit, ZHL-1-2W+), RF switches (mini circuit, ZASWA-2-50DRA), MEMs switches (Sercalo), and delay generators (Stanford Research Systems, DG535).

AFG, it generates two sequential TTL signals to drive the MEMs switch at the output port and a gate signal to turn off the SNSPDs during the AFC preparation time. Finally, from the two remaining marker channels, we use one to generate a 4 MHz clock signal for the time-tagger and another channel to drive Intensity Modulators (IM) and prepare weak coherent probe pulses.

### C. AFC Spectral Hole Burning

To create AFC combs spanning 8 GHz bandwidth, we introduced a new spectral tailoring technique. The procedure combines amplitude and frequency modulation of optical pulses from a narrow-linewidth CW laser, enabling precise manipulation of absorption features. This approach allowed us to achieve broadband squarish AFC structures with background optical depth close to zero for varying storage times.

To date, most QM implementations based on the AFC protocol have used a conventional method to tailor the inhomogeneous broadening described in [2], where a periodic absorbing feature is achieved by employing amplitude and phase modulated optical pulses for optical pumping. Before delving into the preparation of these optical pulses used in the conventional method, we describe a modulated optical pulse that can shape the inhomogeneous broadening to create one spectral hole. Such a pulse can be described by

$$p(t)_{\text{spectral hole}} = \Omega_0[\mathrm{A(t)}]\sin\left[2\pi\nu_0 t + 2\pi\Delta_{ch}[\Phi(t)]\right]. \quad (1)$$

Here, $\Omega_0$ describes the maximum amplitude (Rabi frequency) of the pulse, A(t) and $\Phi(t)$ denotes the desired amplitude and phase modulation functions, $\nu_0$ is the center frequency of the laser, and $\Delta_{ch}$ is the bandwidth of the spectral hole (here the laser linewidth is considered to be very narrow). Considering the periodicity of $\Delta$ in the AFC combs for creating the $n^{th}$ hole, Equation 1 transforms into:

$$p(t)_n = \Omega_0[\mathrm{A(t)}]\sin\left[2\pi(\nu_0 + n\Delta)t + 2\pi\Delta_{ch}[\Phi(t)]\right]. \quad (2)$$

In the conventional method, we prepare a multitone pulse to simultaneously generate $N$ spectral holes periodically. Therefore, we take the summation over all pulses by

$$P(t) = \sum_{n=-\frac{N}{2}}^{\frac{N}{2}} p(t)_n = \sum_{n=-\frac{N}{2}}^{\frac{N}{2}} \Omega_0[\mathrm{A(t)}]\sin\left[2\pi(\nu_0 + n\Delta)t + 2\pi\Delta_{ch}[\Phi(t)]\right]. \quad (3)$$

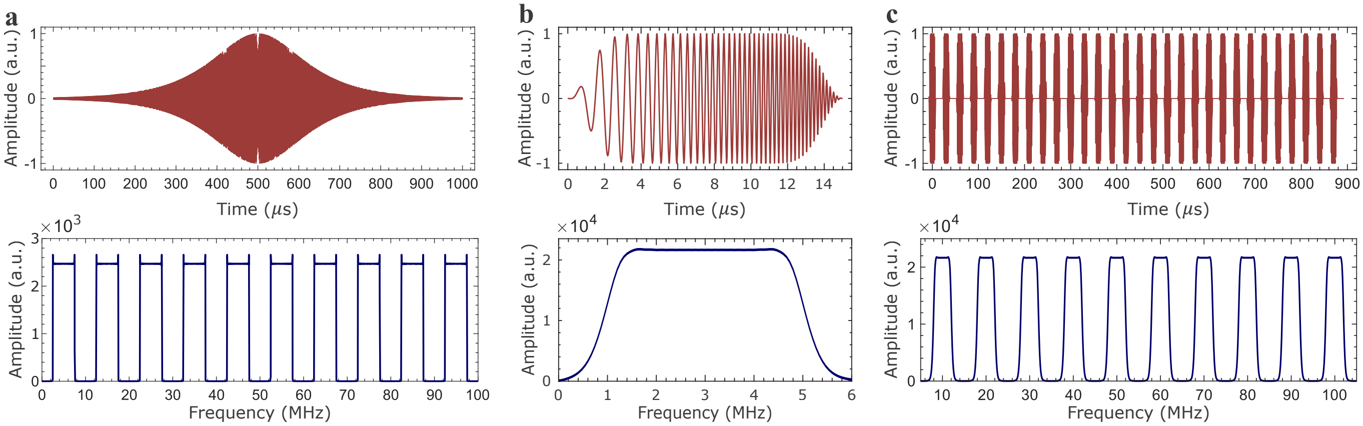


FIG. S3. **Spectral hole tailoring.** **a,** Resulting AFC combs generated with the conventional method described in [2] and Eq. (4). **b,** A 15 $\mu$s WURST pulse described by Eq. (6) is swept over 4 MHz to creating a wide spectral hole. **c,** Application of periodic linearly chirped WURST pulses with 50% duty cycle resulting in a finesse-two AFC comb.

Taking a simpler form, this expression becomes:

$$P(t) = \Omega_0[\mathrm{A(t)}]\frac{\sin(N\pi\Delta t)}{\sin(\pi\Delta t)}\sin\left[2\pi\nu_0 t + 2\pi\Delta_{ch}[\Phi(t)]\right]. \quad (4)$$

The shape of the absorbing features depends highly on the amplitude and phase functions. For example, a complex hyperbolic secant (CHS) pulse [3], which is described by

$$\mathrm{CHS}(t) = \Omega_0 \mathrm{sech}(\beta t)\sin\left[2\pi\nu_0 t + \frac{\pi\Delta_{ch}}{\beta}\ln(\cosh(\beta t))\right], \quad (5)$$

where $\beta = 10/\tau$ is a parameter related to the temporal duration of the pulse, $\tau$, and has a squarish frequency spectrum. This pulse has been utilized in many AFC comb preparations and NMR spectroscopy [4, 5]. An AFC prepared with simultaneous application of CHS pulses results in a multitone pulse (combination of equations 4 and 5) in which the amplitude and frequency spectrum of this pulse are depicted in FIG. S3a.

In addition, wideband, uniform rate, smooth truncation (WURST) pulse with a linear phase sweep also results in a squarish frequency spectrum [6] which is an efficient pulse to transfer population in two-level systems. A linearly swept WURST pulse is described by

$$\mathrm{WURST}(t) = (1 - |\sin(\frac{\pi}{\tau}t)|^M)\times \sin\left[2\pi(\nu_0 + n\Delta)t + 2\pi\frac{\Delta_{ch}}{\tau}t^2\right], \quad (6)$$

in which corresponding amplitude and frequency spectrum are presented in FIG. S3b.

To prepare an AFC comb using WURST pulses, we first determine the number of absorbing teeth within an 8 GHz bandwidth AFC for different storage times, following the relation $N = \Gamma_{\mathrm{AFC}}/\Delta$ or equivalently $N = \Gamma_{\mathrm{AFC}} \times$(storage time). For example, an 8 GHz AFC designed for a 10 ns storage time consists of 80 absorbing teeth, periodically distributed across the AFC bandwidth, while a 100 ns storage time requires 800 periodic absorbing teeth.

To achieve an 8 GHz AFC comb, we generate a train of WURST pulses with a 50% duty cycle using an AOM with the same center frequency for each pulse. Simultaneously, a phase modulator applies a frequency sweep from -3.8 GHz to +4.2 GHz over the entire duration of the pulse train, ensuring proper AFC preparation (i.e., AOM is used for amplitude modulation, while PM is employed for phase modulation). The resulting AFC has a finesse of approximately two, and by adjusting the duty cycle, the finesse can be modified accordingly. In our experiments, the maximum duration of the pulse train is 6 ms, which limits the achievement of longer storage times with 8 GHz AFC bandwidth. This limitation arises because longer storage times require a greater number of absorbing teeth, necessitating more WURST pulses. If the pulse train duration remains fixed, the individual WURST pulses become bandwidth-limited, preventing effective frequency sweeping. Here, FIG. S3c demonstrates the AFC with our method in which is 8.4 times more efficient than the conventional method depicted in the figure FIG. S3a.


[1] See the main article.

[2] M. Businger, L. Nicolas, T. S. Mejia, A. Ferrier, P. Gold-

ner, and M. Afzelius, Non-classical correlations over 1250 modes between telecom photons and 979-nm photons stored in $^{171}Yb^{3+}:Y_2SiO_5$, Nature communications **13**, 6438 (2022).

[3] M. S. Silver, R. I. Joseph, and D. I. Hoult, Selective spin inversion in nuclear magnetic resonance and coherent optics through an exact solution of the Bloch-Riccati equation, Physical review. A, General physics **31**, 2753 (1985).

[4] M. Businger, A. Tiranov, K. T. Kaczmarek, S. Welinski, Z. Zhang, A. Ferrier, P. Goldner, and M. Afzelius, Optical spin-wave storage in a solid-state hybridized electron-nuclear spin ensemble, Physical review letters **124**, 053606 (2020).

[5] R. Siegel, T. T. Nakashima, and R. E. Wasylishen, Sensitivity enhancement of nmr spectra of half-integer spin quadrupolar nuclei in solids using hyperbolic secant pulses, Journal of Magnetic Resonance **184**, 85 (2007).

[6] L. A. O'Dell, The wurst kind of pulses in solid-state nmr, Solid State Nuclear Magnetic Resonance **55–56**, 28–41 (2013).
